# Supplementary material for: On the Convergence of Encoder-only Shallow Transformers
Source: arXiv:2311.01575 source file (2023-11-02)
Supplement: Supplementary file 1 [file appendix_generalization.tex]

% \subsection{Proof of generalization result ( \cref{thm:generalization})}
\begin{algorithm}[h]
\caption{SGD for training \san{} under the NTK initialization}
\label{alg:algorithm_DARTS}
\begin{algorithmic}
\STATE {\bfseries Input:} data $\mathcal{D}_{tr} = \{ (\mX_n, y_n)_{i=1}^N \}$, step size $\gamma$.\\
\STATE   NTK initialization for the weights based on \cref{tab:init}.
\STATE
$\mW^0_Q \sim \mathcal{N}
% (0,1/{d})
(0,1)
$,
$\mW^0_K \sim \mathcal{N}
% (0,1/{d})
(0,1)
$,
\STATE
$\mW^0_V \sim \mathcal{N}
% (0,1/{d})
(0,1)
$,
$\mW^0_O \sim \mathcal{N}
% (0,1/{d_m})
(0,1)
$.
\\
\STATE Construct the \san{} $f(\mX; \wall^0)$ based on $\mW_Q^{0},\mW_K^{0},\mW_V^{0},\mW_O^{0}$. 
\FOR{$n=0$ {\bfseries to} $N-1$}
\STATE{$\wall^{n+1} = \wall^{n}- \gamma\cdot \nabla_{\wall} \ell \big( f(\mX_n; \wall^{n}) y_n \big)\,.$} 
\ENDFOR \\
\textbf{Output}  Randomly choose $\hat{\wall}$ uniformly from $\left \{ \wall^{0}, \dots , \wall^{N-1} \right \} $.
\end{algorithmic}
\end{algorithm}
\label{sec:proof_generalization}
In this section, we present the proof for the generalization result on \cref{thm:generalization}. Firstly, we provide some useful lemmas.
\begin{lemma}
\label{lemma:bound_for_perturbation}
Given an initial weight vector $\mW \in \R^{d_m \times d}$, where $d_m>d$, each element is sampled independently from $\mathcal{N}(0, 1)$, for any $\tilde \mW$ such that $\|\tilde \mW-\mW\|_2 \le R$, with probability at least $1-2\exp(-{d_m}/{2})$, one has:
\begin{equation}
    \|\tilde \mW\|_2
\le 
    R+3\sqrt{d_m}\,.
    \end{equation}
\end{lemma}
\begin{proof}
By triangle inequality and \cref{lemma:gaussl2}:
    \begin{equation}
    \|\tilde \mW\|_2
\le 
    \|\tilde \mW\ -\mW \|_2+    \|\mW\|_2
\le 
    R+3\sqrt{d_m}\,.
    \end{equation}
\end{proof}
\begin{lemma} The output of the last second layer can be upper bounded by:
$
\norm{\vf_\text{pre}(\mX;\mW)}_2 \leq \tau_1 d_s \norm{\mW_V}_2 C_x.$
\label{lemma:boundf}
\end{lemma}
\begin{proof}
    \begin{equation}
        \begin{split}
  &  \norm{\vf_\text{pre}(\mX;\mW)}_2
    =\norm{
     \tau_1 
    \sum_{i=1}^{d_s}
    \sigma_r
    \left(
    \mW_V\mX^\top \vbeta_i  
    % \vf_\text{first}
    \right)
    }_2
 \leq
 \tau_1 d_s
     \norm{
        \sigma_r
        \left(
        \mW_V\mX^\top \vbeta_i  
        % \vf_\text{first}
        \right)
        }_2
  \leq
      \tau_1 d_s \norm{\mW_V}_2 C_x
        \end{split}
    \end{equation}
\end{proof}

The lemma below shows that if the weights are close, the output of each neuron does not change too much.
\begin{lemma}[Bound of $        \norm{  \vf_\text{pre}^\prime(\mX;\mW)
        -
        \vf_\text{pre}(\mX;\mW)}_2$]
\label{lemma:boundfminusf}
\end{lemma}
\begin{proof}
    \begin{equation}
        \begin{split}
        &       \norm{  \vf_\text{pre}^\prime(\mX;\mW)
        -
        \vf_\text{pre}(\mX;\mW)}_2
 =
 \norm{\tau_1 
    \sum_{i=1}^{d_s}
    \sigma_r
    \left(
    \mW_V^\prime\mX^\top \vbeta_i^\prime
    \right)-
    \tau_1 
    \sum_{i=1}^{d_s}
    \sigma_r
    \left(
    \mW_V\mX^\top \vbeta_i  
    \right)}
\\& \leq
  \tau_1 d_s \norm{\mW_V^\prime\mX^\top \vbeta_1^\prime-\mW_V\mX^\top \vbeta_1}_2
   \leq
  \tau_1 d_s \norm{\mW_V^\prime-\mW_V}_2 \norm{\mX}_2 \norm{\vbeta_1^\prime-\vbeta_1}_2
   \leq
     2 \tau_1 d_sC_x  \norm{\mW_V^\prime-\mW_V}_2 
        \end{split}
    \end{equation}
\end{proof}
We also need the following lemma, demonstrating that when the initializations are close to each other, the \san{} is almost linear in terms of its weights.
\begin{lemma}
\label{lemma:lemma_4.1_in_GuQuanquan}
Let $\mW' \in \mathcal{B} (\mW,\omega )$  with $\omega = \mathcal{O}
% ((3\mathrm{Lip}_{\max}+1)^{-(L-1)})
(1)
$ 
,
% for any $i \in [N]$,
with probability at least $1-8\exp(-d_m/2)$, we have:
\begin{equation*}
\left | f(\mX;\mW') - f(\mX;\mW) - \left \langle \nabla  f(\mX;\mW), \mW' -\mW  \right \rangle \right | = \mathcal{O}(1)\,.
\end{equation*}
\end{lemma}
\begin{proof}
\label{proof:lemma_4.1_in_GuQuanquan}
We have the following expression:
\begin{equation}
\small
\begin{split}
& 
    \left | f(\mX;\mW') - f(\mX;\mW) - \left \langle \nabla  f(\mX;\mW), \mW' -\mW  \right \rangle \right | 
\\ & = 
         \left |
   \vw_O^{\prime\top}
        (
        \vf_\text{pre}^\prime(\mX;\mW)
        -
        \vf_\text{pre}(\mX;\mW)
        )
        -
        \langle \nabla  f_{\mW_V}(\mX;\mW),
    \mW_V' -\mW_V\rangle
        -
            \langle \nabla  f_{\mW_Q}(\mX;\mW),
    \mW_Q' -\mW_Q\rangle
        -
        \langle \nabla  f_{\mW_K}(\mX;\mW),
    \mW_K' -\mW_K\rangle
    \right | 
\\ & \leq
         \norm{ \vw_O^{\prime}}_2
        \norm{  \vf_\text{pre}^\prime(\mX;\mW)
        -
        \vf_\text{pre}(\mX;\mW)}_2
        +
        \norm{\nabla  f_{\mW_V}(\mX;\mW)}_2
        \norm{\mW_V' -\mW_V}_2
 \\ &\qquad +
        \norm{\nabla  f_{\mW_Q}(\mX;\mW)} _2
        \norm{\mW_Q' -\mW_Q}_2
                +
        \norm{\nabla  f_{\mW_K}(\mX;\mW)} _2
        \norm{\mW_K' -\mW_K}_2
\end{split}
\label{eq:proof_lemma_4.1_in_GuQuanquan_1}
\end{equation}

By~\cref{thm:inequality_initialization},
with probability at least $1-8\exp(-d_m/2)$, we have 
$\left \|\mW_Q\right \|_2 \leq 3\sqrt{\eta_{Q} d_m}$,
$\left \|\mW_K\right \|_2 \leq 3\sqrt{\eta_{K} d_m}$,
$\left \|\mW_V\right \|_2 \leq 3\sqrt{\eta_V d_m}$,
$\left \|\vw_O\right \|_2 \leq 3\sqrt{\eta_O d_m}$.

The first term of \cref{eq:proof_lemma_4.1_in_GuQuanquan_1} can be bounded with probability at least $1-8\exp(-d_m/2)$ as follows:
\begin{equation}
    \begin{split}
&
                \norm{ \vw_O^{\prime}}_2
        \norm{  \vf_\text{pre}^\prime(\mX;\mW)
        -
        \vf_\text{pre}(\mX;\mW)}_2
\\ & \leq 
    \norm{ \vw_O^{\prime}}_2 2\tau_1 d_sC_x  \norm{\mW_V^\prime-\mW_V}_2
   \quad \mbox{(By \cref{lemma:boundfminusf})}
\\ & \leq 
    (3 \sqrt{\eta_O d_m}+\omega) 2\tau_1 d_sC_x  \omega
    \end{split}
\end{equation}

The second term of \cref{eq:proof_lemma_4.1_in_GuQuanquan_1} can be bounded with probability at least $1-8\exp(-d_m/2)$ as follows:
\begin{equation}
    \begin{split}
&   \norm{\nabla  f_{\mW_V}(\mX;\mW)}_2
        \norm{\mW_V' -\mW_V}_2
\\ & \leq 
    \omega  \norm{\nabla  f_{\mW_V}(\mX;\mW)}_2
\\ & \leq 
    \omega  \tau_1
     d_s
    \norm{\vw_O}_2
    C_x
   \quad \mbox{(By \cref{lemma:gradientbound})}
\\ & \leq 
   3\sqrt{\eta_O d_m}  \omega  \tau_1
     d_s
    C_x
    \end{split}
\end{equation}

The third term of \cref{eq:proof_lemma_4.1_in_GuQuanquan_1} can be bounded with probability at least $1-8\exp(-d_m/2)$ as follows:
\begin{equation}
    \begin{split}
&   \norm{\nabla  f_{\mW_Q}(\mX;\mW)}_2
        \norm{\mW_Q' -\mW_Q}_2
\\ & \leq 
    \omega  \norm{\nabla  f_{\mW_Q}(\mX;\mW)}_2
\\ & \leq 
    \omega 
    2 
    \tau_0 \tau_1
        d_s 
    \norm{\mW_K}_2
        \norm{\mW_V}_2
            \norm{\vw_O}_2
    C_x^3
   \quad \mbox{(By \cref{lemma:gradientbound})}
\\ & \leq 
 2 (3 \sqrt{\eta_O d_m})
 (3 \sqrt{\eta_K d_m})
 (3 \sqrt{\eta_V d_m})
 \omega \tau_0 \tau_1  C_x^3
    \end{split}
\end{equation}
Similarly, the fourth term of \cref{eq:proof_lemma_4.1_in_GuQuanquan_1} can be bounded with probability at least $1-8\exp(-d_m/2)$ as follows:
\begin{equation}
    \begin{split}
&   \norm{\nabla  f_{\mW_K}(\mX;\mW)}_2
        \norm{\mW_K' -\mW_K}_2
\leq 
 2 (3 \sqrt{\eta_O d_m})
 (3 \sqrt{\eta_Q d_m})
 (3 \sqrt{\eta_V d_m})
 \omega \tau_0 \tau_1  C_x^3
    \end{split}
\end{equation}

% Moreover, $m\left \| \mW_{L} \right \|_2^2$ is a random Variables obey chi-square distribution with $m$ degrees of freedom. That means $\mathbb{E} (m\left \| \mW_{L} \right \|_2^2)=m$ and $\mathbb{V}(m\left \| \mW_{L} \right \|_2^2)=2m$. By Chebyshev's Inequality we have $P(|m\left \| \mW_{L} \right \|_2^2-m|\geq m)\leq 2m/m^{2}$. i.e.:
% \begin{equation*}
% \left \| \mW_{L} \right \|_2\leq \sqrt{2}\,,
% \end{equation*}
% with probability at least $1-2/m$.
 
Accordingly, under the setting of NTK's initialization, i.e., $\eta_V = \eta_{Q}=\eta_{K} =\eta_O = 1$, $\tau_0=\frac{1}{d_m}$, $\tau_1=\frac{1}{\sqrt{d_m}}$,~\cref{eq:proof_lemma_4.1_in_GuQuanquan_1} can be further bounded with probability at least $1-8\exp(-d_m/2)$ as follows:
\begin{equation*}
\begin{split}
    & \left | f(\mX;\mW') - f(\mX;\mW) - \left \langle \nabla  f(\mX;\mW), \mW' -\mW  \right \rangle \right | = \mathcal{O}(1)\,.
\end{split}
\end{equation*}
\end{proof}

Let us define $L(\bm{W})  = \ell[ y f(\mX;\bm{W}) ]$, the following lemma shows that, $L(\bm{W})$ is almost a convex function of $\bm{W}$ 
% for any $i \in [N]$ 
if the weights are close to the one at the initialization.
\begin{lemma}
\label{lemma:lemma_4.2_in_GuQuanquan}
Let $ \bm{W}' \in \mathcal{B} (\bm{W},\omega )$  with $\omega = \mathcal{O}(1)$, it holds that:
\begin{equation*}
L(\bm{W}') \geq L(\bm{W}) + \left \langle \nabla_{\bm{W}} L(\bm{W}), \bm{W}'-\bm{W} \right \rangle -\mathcal{O}(1)\,,
\end{equation*}
with probability at least $1-8\exp(-m/2)$.
\end{lemma}
\begin{proof}
\label{proof:lemma_4.2_in_GuQuanquan}
By the convexity of $\ell(z)$, one has:
\begin{equation*}
\small
    L({\bm{W}}') - L(\bm{W}) =  \ell[y  f(\mX;{\bm{W}}') ] - \ell[ y f(\mX;\bm{W}) ] \geq  \ell'[ y f(\mX;\bm{W})] \cdot y\cdot [ f(\mX;{\bm{W}}') - f(\mX;\bm{W}) ]\,.
\end{equation*}
By the chain rule:
\begin{align*}
&\left \langle  \nabla_{\bm{W}_Q} L(\bm{W}), \bm{W}_Q' - \bm{W}_Q  \right \rangle
    +
        \left \langle  \nabla_{\bm{W}_K} L(\bm{W}), \bm{W}_K' - \bm{W}_K  \right \rangle
    +
        \left \langle  \nabla_{\bm{W}_V} L(\bm{W}), \bm{W}_V' - \bm{W}_V  \right \rangle
    +
            \left \langle  \nabla_{\bm{w}_o} L(\bm{W}), \bm{w}_O' - \bm{w}_O  \right \rangle
 \\&= \ell'[ y f(\mX;\bm{W})] \cdot y\cdot \left \langle  \nabla f(\mX;\bm{W}) , {\bm{W}}' - \bm{W} \right \rangle\,.
\end{align*}
Combining the above two equations, and using the triangle inequality, one has:
\begin{equation*}
\small
\begin{split}
       & \ell'[ y f(\mX;\bm{W})]\cdot y\cdot[ f(\mX;{\bm{W}}') - f(\mX;\bm{W}) ]  \geq \ell'[ y f(\mX;\bm{W})] \cdot y\cdot  \left \langle  \nabla f(\mX;\bm{W}) , {\bm{W}}' - \bm{W}  \right \rangle   - \varepsilon \\
& = \textstyle  
    \left \langle  \nabla_{\bm{W}_Q} L(\bm{W}), \bm{W}_Q' - \bm{W}_Q  \right \rangle
    +
        \left \langle  \nabla_{\bm{W}_K} L(\bm{W}), \bm{W}_K' - \bm{W}_K  \right \rangle
    +
        \left \langle  \nabla_{\bm{W}_V} L(\bm{W}), \bm{W}_V' - \bm{W}_V  \right \rangle
    +
            \left \langle  \nabla_{\bm{w}_o} L(\bm{W}), \bm{w}_O' - \bm{w}_O  \right \rangle
    - \varepsilon\,,
\end{split}
\end{equation*}
where $\varepsilon := | \ell'[ y f(\mX;\bm{W})] \cdot y\cdot [ f(\mX;{\bm{W}}') - f(\mX;\bm{W})  - \left \langle \nabla f(\mX;\bm{W}) , {\bm{W}}' - \bm{W} \right \rangle ] |$.  Lastly, according to the upper-bounding $\varepsilon$ with~\cref{lemma:lemma_4.1_in_GuQuanquan} and the fact that $| \ell'[ y f(\mX;\bm{W})] \cdot y | \leq 1$, one has:
\begin{equation*}
\begin{split}
 &    L({\bm{W}}') - L(\bm{W})  \\&\geq     \left \langle  \nabla_{\bm{W}_Q} L(\bm{W}), \bm{W}_Q' - \bm{W}_Q  \right \rangle
    +
        \left \langle  \nabla_{\bm{W}_K} L(\bm{W}), \bm{W}_K' - \bm{W}_K  \right \rangle
    +
        \left \langle  \nabla_{\bm{W}_V} L(\bm{W}), \bm{W}_V' - \bm{W}_V  \right \rangle
    +
            \left \langle  \nabla_{\bm{w}_o} L(\bm{W}), \bm{w}_O' - \bm{w}_O  \right \rangle
    - \varepsilon\\
     & =     \left \langle  \nabla_{\bm{W}_Q} L(\bm{W}), \bm{W}_Q' - \bm{W}_Q  \right \rangle
    +
        \left \langle  \nabla_{\bm{W}_K} L(\bm{W}), \bm{W}_K' - \bm{W}_K  \right \rangle
    +
        \left \langle  \nabla_{\bm{W}_V} L(\bm{W}), \bm{W}_V' - \bm{W}_V  \right \rangle
    +
            \left \langle  \nabla_{\bm{w}_o} L(\bm{W}), \bm{w}_O' - \bm{w}_O  \right \rangle - \mathcal{O}(1)\,.
\end{split}
\end{equation*}
\end{proof}
The following lemma aims to show that the gradient of the neural network can be upper bounded when the weights are close to initialization.
\begin{lemma}
\label{lemma:lemma_B.3_in_GuQuanquan}
Let $\bm{W}^\prime \in \mathcal{B} (\bm{W},\omega )$   with $\omega = \mathcal{O}(1)$, with probability at least $1-8\exp(-m/2)$, it holds that:
\begin{equation*}
\left \| \nabla_{\bm{W}_Q^\prime} L(\mX;\bm{W}^\prime) \right \| _2,
\left \| \nabla_{\bm{W}_K^\prime} L(\bm{W}^\prime) \right \| _2 ,
\left \| \nabla_{\bm{W}_V^\prime} L(\bm{W}^\prime) \right \| _2 ,
\left \| \nabla_{\vw_O^\prime} L(\bm{W}^\prime) \right \| _2 
\leq  \mathcal{O}(1)\,.
\end{equation*}

\end{lemma}

\begin{proof}
\label{proof:lemma_B.3_in_GuQuanquan}
By the gradient in \cref{lemma:gradientbound}, with probability at least $1-8\exp(-m/2)$, one has:
\begin{equation*}
\begin{split}
& \norm{ \nabla_{\bm{W}_V^\prime} 
 f(\mX;\bm{W}^\prime) }_2
\leq
    \tau_1
     d_s
    \norm{\vw_O}_2
    C_x
   % \quad \mbox{(By }
\leq 
   (3\sqrt{\eta_O d_m}+  \omega)  \tau_1
     d_s
\end{split}
\end{equation*}
\begin{equation*}
\begin{split}
& \norm{ \nabla_{\vw_O^\prime} 
 f(\mX;\bm{W}^\prime) }_2
\leq
\tau_1
     d_s
    \norm{\mW_V^\prime}_2
    C_x
    % \quad \mbox{(By \cref{lemma:gradientbound})}
\leq
     (3\sqrt{\eta_V d_m}+  \omega)
     \tau_1
     d_s
    C_x
\end{split}
\end{equation*}
\begin{equation*}
\begin{split}
& \norm{ \nabla_{\bm{W}_Q^\prime} 
 f(\mX;\bm{W}^\prime) }_2
\leq 
    2 
    \tau_0 \tau_1
        d_s 
    \norm{\mW_K^\prime}_2
        \norm{\mW_V^\prime}_2
            \norm{\vw_O^\prime}_2
    C_x^3
   % \quad \mbox{(By \cref{lemma:gradientbound})}
 \leq 
 2 (3 \sqrt{\eta_O d_m}+\omega)
 (3 \sqrt{\eta_{K} d_m}+\omega)
 (3 \sqrt{\eta_V d_m}+\omega)
\tau_0 \tau_1  C_x^3
\end{split}
\end{equation*}
\begin{equation*}
\begin{split}
& \norm{ \nabla_{\bm{W}_K^\prime} 
 f(\mX;\bm{W}^\prime) }_2
\leq 
 2 (3 \sqrt{\eta_O d_m}+\omega)
 (3 \sqrt{\eta_{Q} d_m}+\omega)
 (3 \sqrt{\eta_V d_m}+\omega)
\tau_0 \tau_1  C_x^3
\end{split}
\end{equation*}

Under the setting of NTK's initialization, we can easily see that 
\begin{equation*}
\left \| \nabla_{\bm{W}_Q^\prime} f(\mX;\bm{W}^\prime) \right \| _2,
\left \| \nabla_{\bm{W}_K^\prime} f(\bm{W}^\prime) \right \| _2 ,
\left \| \nabla_{\bm{W}_V^\prime} f(\bm{W}^\prime) \right \| _2 ,
\left \| \nabla_{\vw_O^\prime} f(\bm{W}^\prime) \right \| _2 
\leq  \mathcal{O}(1)\,.
\end{equation*}
Furthermore,
\begin{equation*}
\small
\left \| \nabla_{\bm{W}_Q^\prime} L(\bm{W}^\prime) \right \| _2 \leq \left | {\ell}'[y\cdot f(\mX;\bm{W})]\cdot y\right | \cdot \left \| \nabla_{\bm{W}_Q^\prime} f(\mX;\bm{W}^\prime) \right \| _2 \leq \left \| \nabla_{\bm{W}_Q^\prime} f(\mX;\bm W^\prime) \right \| _2 \leq  \mathcal{O}(1),
\end{equation*}
where we use the fact that $| \ell'[ yf(\mX;\bm{W})] \cdot y| \leq 1$.
Similarly, we can obtain the remaining result and complete the proof.
\end{proof}

We need the following lemma to show that, the cumulative loss can be upper bounded under small changes on the parameters (i.e., weights).  
\begin{lemma}
\label{lemma:lemma_4.3_in_GuQuanquan}
    For any $\epsilon, \delta, R > 0$, there exists:
   $
    m^{\star}= \frac{R^4}{4\varepsilon^2}\,,
    $
    such that if $m \geq m^* (\epsilon, \delta, R,L)$, then with probability at least $1 - \delta$ over the randomness of $\mW^0$, for any $\bm{W}^* \in \mathcal{B} (\mW^0, R m^{-1/2})$, with step size $\gamma = \varepsilon/{d_m}$, $N = R^2/(2\varepsilon^2)$, the cumulative loss can be upper bounded by:
    \begin{equation*}
        \sum_{n=0}^{N-1} L_n(\mW^n) \leq \sum_{n=0}^{N-1} L_n(\bm{W}^{*}) + 3N\epsilon\,.
    \end{equation*}
\end{lemma}
\begin{proof}
Set $\omega = 1$ such that the conditions on $\omega$ given in Lemmas~\ref{lemma:lemma_4.1_in_GuQuanquan},~\ref{lemma:lemma_4.2_in_GuQuanquan} and~\ref{lemma:lemma_B.3_in_GuQuanquan} hold. It is easy to see that as long as $m \geq R^2$, we have $\bm{W}^* \in \mathcal{B} (\mW^0, \omega)$. 
We now show that under our parameter choice, 
$\mW^0,\ldots,\mW^{N-1} $ are inside $ \mathcal{B} (\mW^0, \omega)$ as well. 

This result follows by simple induction. Clearly we have $\mW^0 \in \mathcal{B} (\mW^0, \omega)$. Suppose that $ \mW^0,\ldots, \mW^n \in \mathcal{B} (\mW^0, \omega) $. Then by~\cref{lemma:lemma_B.3_in_GuQuanquan}, we have 
$
\|\nabla_{{\bm{W}}_Q} L_n(\mW^n)\|_2,
\|\nabla_{{\bm{W}}_K} L_n(\mW^n)\|_2,
\|\nabla_{{\bm{W}}_V} L_n(\mW^n)\|_2,
\|\nabla_{{\bm{W}}_O} L_n(\mW^n)\|_2
\leq \Theta(1).
$

Therefore:
\begin{align*}
 &
    \big\| \bm{W}_Q^{n+1} - \bm{W}_Q^{0} \big\|_2 \leq \sum_{j  = 0}^i\big\| \bm{W}_Q^{j+1} - \bm{W}_Q^{j} \big\|_2 \leq \Theta(\gamma N)\,,
\quad
    \big\| \bm{W}_K^{n+1} - \bm{W}_K^{0} \big\|_2 \leq \sum_{j  = 0}^i\big\| \bm{W}_K^{j+1} - \bm{W}_K^{j} \big\|_2 \leq \Theta(\gamma N)\,,
\\ &
    \big\| \bm{W}_V^{n+1} - \bm{W}_V^{0} \big\|_2 \leq \sum_{j  = 0}^i\big\| \bm{W}_V^{j+1} - \bm{W}_V^{j} \big\|_2 \leq \Theta(\gamma N)\,,
\quad
    \big\| \vw_O^{n+1} - \vw_O^{0} \big\|_2 \leq \sum_{j  = 0}^i\big\| \vw_O^{j+1} - \vw_O^{j} \big\|_2 \leq \Theta(\gamma N)\,,
\end{align*}
Plugging in our parameter choice 
$\gamma = \varepsilon/{d_m}$, $N = R^2/(2\varepsilon^2)$, then if $d_m \geq R^4/(4\varepsilon^2)$, one has:
% for some small enough absolute constant $\nu$
\begin{align*}
&
    \big\| \bm{W}_Q^{n+1} - \bm{W}_Q^{0} \big\|_{\mathrm{F}} \leq\Theta\bigg(\sqrt{d_m}\frac{R^2}{2d_m\varepsilon}\bigg) \leq \omega\,,
\quad
    \big\| \bm{W}_K^{n+1} - \bm{W}_K^{0} \big\|_{\mathrm{F}} \leq\Theta\bigg(\sqrt{d_m}\frac{R^2}{2d_m\varepsilon}\bigg) \leq \omega\,,
\\ &
    \big\| \bm{W}_V^{n+1} - \bm{W}_V^{0} \big\|_{\mathrm{F}} \leq\Theta\bigg(\sqrt{d_m}\frac{R^2}{2d_m\varepsilon}\bigg) \leq \omega\,,
\quad
    \big\| \vw_O^{n+1} - \vw_O^{0} \big\|_{\mathrm{F}} \leq\Theta\bigg(\sqrt{d_m}\frac{R^2}{2d_m\varepsilon}\bigg) \leq \omega\,,
\end{align*}
Therefore by induction we see that $\mW^0,\ldots,\mW^{N-1} \in \mathcal{B} (\mW^0, \omega)$. As a result, the conditions of Lemmas~\ref{lemma:lemma_4.1_in_GuQuanquan},~\ref{lemma:lemma_4.2_in_GuQuanquan} and~\ref{lemma:lemma_B.3_in_GuQuanquan} are satisfied for $\bm{W}^*$ and $\mW^0,\ldots, \mW^{N-1}$.

Next, we utilize the results of Lemmas~\ref{lemma:lemma_4.1_in_GuQuanquan},~\ref{lemma:lemma_4.2_in_GuQuanquan} and~\ref{lemma:lemma_B.3_in_GuQuanquan} to prove the bound of cumulative loss. First of all, by~\cref{lemma:lemma_4.2_in_GuQuanquan}, we have:
\begin{equation*}
\begin{split}
\small
&
    L_n(\mW^n) - L_n(\bm{W}^{*}) 
\leq
    \left \langle  \nabla_{\bm{W}} L_n(\mW^n), \mW^n - \bm{W}^*  \right \rangle  + \epsilon 
\\&= 
    \frac{\left \langle  \bm{W}_Q^n - \bm{W}_Q^{n+1}, \bm{W}_Q^n - \bm{W}_Q^*  \right \rangle  }{ \gamma }
    +
    \frac{\left \langle  \bm{W}_K^n - \bm{W}_K^{n+1}, \bm{W}_K^n - \bm{W}_K^*  \right \rangle  }{ \gamma }
\\&\quad \quad
    +
    \frac{\left \langle  \bm{W}_V^n - \bm{W}_V^{n+1}, \bm{W}_V^n - \bm{W}_V^*  \right \rangle  }{ \gamma }
    +
    \frac{\left \langle  \vw_O^n - \vw_O^{n+1}, \vw_O^n - \vw_O^*  \right \rangle  }{ \gamma }
    + \epsilon\,.
\end{split}
\end{equation*}
Note that for the matrix inner product we have the equality $2\left \langle \bm{A},\bm{B} \right \rangle = \left \| \bm{A} \right \| _{\mathrm{F}}^2 + \left \| \bm{B} \right \| _{\mathrm{F}}^2 - \left \| \bm{A-B} \right \| _{\mathrm{F}}^2$. Applying this equality to the right hand side above provides:
\begin{equation*}
\small
\begin{split}
&    
    L_n(\mW^n) - L_n(\bm{W}^{*}) 
\\&\leq 
    \frac{ \| \bm{W}_Q^n - \bm{W}_Q^{n+1} \|_{\mathrm{F}}^2 + \| \bm{W}_Q^n - \bm{W}_Q^* \|_{\mathrm{F}}^2 - \| \bm{W}_Q^{n+1} - \bm{W}_Q^* \|_{\mathrm{F}}^2 } {2\gamma} 
    +
        \frac{ \| \bm{W}_K^n - \bm{W}_K^{n+1} \|_{\mathrm{F}}^2 + \| \bm{W}_K^n - \bm{W}_K^* \|_{\mathrm{F}}^2 - \| \bm{W}_K^{n+1} - \bm{W}_K^* \|_{\mathrm{F}}^2 } {2\gamma} 
\\&  \quad  +
        \frac{ \| \bm{W}_V^n - \bm{W}_V^{n+1} \|_{\mathrm{F}}^2 + \| \bm{W}_V^n - \bm{W}_K^* \|_{\mathrm{F}}^2 - \| \bm{W}_V^{n+1} - \bm{W}_V^* \|_{\mathrm{F}}^2 } {2\gamma} 
    +
        \frac{ \| \vw_O^n - \vw_O^{n+1} \|_{\mathrm{F}}^2 + \| \vw_O^n - \vw_O^* \|_{\mathrm{F}}^2 - \| \vw_O^{n+1} - \vw_O^* \|_{\mathrm{F}}^2 } {2\gamma} 
    +
    \epsilon\,.
\end{split}
\end{equation*}
By~\cref{lemma:lemma_B.3_in_GuQuanquan}, we have $$\| \bm{W}_Q^n - \bm{W}_Q^{n+1} \|_{\mathrm{F}} \leq \gamma\sqrt{d_m}\|\nabla_{\bm{W}_Q} L_n(\mW^n)\|_2 \leq \Theta (\gamma\sqrt{d_m}).$$
Similarly:
$$\| \bm{W}_K^n - \bm{W}_K^{n+1} \|_{\mathrm{F}},
\| \bm{W}_V^n - \bm{W}_V^{n+1} \|_{\mathrm{F}},
\| \vw_O^n - \vw_O^{n+1} \|_{\mathrm{F}}
\leq \Theta (\gamma\sqrt{d_m}).$$

Therefore:
\begin{equation*}
\begin{split}   
\small
&    L_n(\mW^n) - L_n(\bm{W}^{*}) 
\\ & \leq 
    \frac{ \| \bm{W}_Q^n - \bm{W}_Q^* \|_{\mathrm{F}}^2 - \| \bm{W}_Q^{n+1} - \bm{W}_Q^* \|_{\mathrm{F}}^2 } {2\gamma}
    +
        \frac{ \| \bm{W}_K^n - \bm{W}_K^* \|_{\mathrm{F}}^2 - \| \bm{W}_K^{n+1} - \bm{W}_K^* \|_{\mathrm{F}}^2 } {2\gamma}
\\ &    +
        \frac{ \| \bm{W}_V^n - \bm{W}_V^* \|_{\mathrm{F}}^2 - \| \bm{W}_V^{n+1} - \bm{W}_V^* \|_{\mathrm{F}}^2 } {2\gamma}
    +
        \frac{ \| \vw_O^n - \vw_O^* \|_{\mathrm{F}}^2 - \| \vw_O^{n+1} - \vw_O^* \|_{\mathrm{F}}^2 } {2\gamma}
    +
    \Theta (\gamma m) + \epsilon\,.
\end{split} 
\end{equation*}
Telescoping over $n = 0,\ldots, N-1$, we obtain:
\begin{equation*}
\small
\begin{split} 
& 
    \frac{1}{N}\sum_{n=0}^{N-1} L_n(\mW^n)
\\&\leq
    \frac{1}{N}\sum_{n=0}^{N-1} L_n(\bm{W}^{*}) + \frac{ 
    \| \bm{W}_Q^{0} - \bm{W}_Q^* \|_{\mathrm{F}}^2 
    +
    \| \bm{W}_K^{0} - \bm{W}_K^* \|_{\mathrm{F}}^2 
    +
    \| \bm{W}_V^{0} - \bm{W}_V^* \|_{\mathrm{F}}^2 
    +
    \| \vw_O^{0} - \vw_O^* \|_{\mathrm{F}}^2 
    } {2N\gamma} + \Theta (\gamma m) + \epsilon
\\&\leq
    \frac{1}{N}\sum_{n=0}^{N-1} L_n(\bm{W}^{*}) + \frac{ L R^{2} } {2\gamma mN} + \Theta (\gamma m) + \epsilon\,,
\end{split} 
\end{equation*}
where the second inequality follows by the assumption that $\bm{W}^*\in \mathcal{B} (\mW^0,Rm^{-1/2})$. 
Plugging in the parameter choice 
$\gamma = \varepsilon/{d_m}$, $N = R^2/(2\varepsilon^2)$, then:
\begin{align*}
    \frac{1}{N}\sum_{n=0}^{N-1} L_n(\mW^n) &\leq \frac{1}{N}\sum_{n=0}^{N-1} L_n(\bm{W}^{*}) + 3\epsilon\,,
\end{align*}
which finishes the proof.
\end{proof}
Now we are ready to finish the proof of ~\cref{thm:generalization}.
\begin{proof}
By Lemmas~\ref{lemma:lemma_4.1_in_GuQuanquan},~\cref{lemma:lemma_4.3_in_GuQuanquan} and Theorem 3.3, Lemma 4.4, Corollary 3.10 in ~\citep{cao2019generalization}, 
% let $C_1(L) = \sqrt{L}/(3\mathrm{Lip}_{\max}+1)^{L-1}$ and $C_2(L) = \sqrt{L}(3\mathrm{Lip}_{\max}+1)^{L-1}$, bring in our $\gamma$ and $N$ with a not very large $L$, 
we have:
\begin{equation*}
\mathbb{E}[\ell_{\mathcal{D} }^{0-\!1}\!(\hat{\bm{W}}\!)] \!\leq\! \tilde{\mathcal{O} }\! \left(\! \sqrt{\frac{\vy^{\top}  ({\bm{K}^\star})^{-1} \vy}{N}} \!\right) + \mathcal{O}\!\left( \! \sqrt{\frac{\log(1/\delta )}{N} } \! \right)\!.
\end{equation*}

According to the courant minimax principle~\citep{10.5555/248979}: $\frac{1}{\lambda_{\min}(\mK^\star)} =\lambda_{\max}(({\mK^\star})^{-1}) = \max \frac{\vy^{\top}({\mK^\star})^{-1})\vy}{\vy^{\top}\vy}$, that means $\vy^{\top}(({\mK^\star})^{-1})\vy \leq \frac{\vy^{\top}\vy}{\lambda_{\min}(\mK^\star)}$, then we have the final bound:

\begin{equation*}
\mathbb{E}[\ell_{\mathcal{D} }^{0-\!1}\!(\hat{\bm{W}}\!)] \!\leq\! \tilde{\mathcal{O} }\! \left(\! C_2\sqrt{\frac{\vy^{\top}\vy}{\lambda_{\min}(\mK^\star) N}} \!\right) + \mathcal{O}\!\left( \! \sqrt{\frac{\log(1/\delta )}{N} } \! \right)\!.
\end{equation*}
\end{proof}
